# Supplementary material for: When Prompts Ignore Structure: Graph-Based Attribute Reasoning for Calibrated VLMs
Source: arXiv:2607.07395 source file (2026-07-28)
Supplement: Supplementary file 2 [file 7_appendix_index.tex]

\begin{table*}[t]
\centering

\setlength{\tabcolsep}{6pt}
\caption*{\large\textbf{Appendix Contents}}
\begin{tabular}{@{}p{0.72\linewidth}r@{}}
\toprule
\textbf{Section} & \textbf{Page} \\
\midrule

% ── Datasets ──────────────────────────────────────────
\hyperref[datasets]{\textbf{A\; Datasets}}
  & \pageref{datasets} \\[4pt]

% ── GAT Architecture ──────────────────────────────────
\hyperref[app:architecture]{\textbf{B\; GAT Architecture Details}}
  & \pageref{app:architecture} \\
\quad\hyperref[app:architecture]{\textit{Attention and Aggregation}}
  & \pageref{app:architecture} \\
\quad\hyperref[app:architecture]{\textit{Residual, Normalisation, and Projection}}
  & \pageref{app:architecture} \\
\quad\hyperref[app:architecture]{\textit{Node Attention Score}}
  & \pageref{app:architecture} \\[4pt]

% ── Ablation Studies ──────────────────────────────────
\hyperref[app:ablation]{\textbf{C\; Ablation Studies}}
  & \pageref{app:ablation} \\
\quad\hyperref[app:ablation]{\textit{C.1\; Attribute Comparison: TCA vs.\ \ARGTCADiv{} vs.\ \ARGTCADisc{}}}
  & \pageref{app:ablation} \\
\quad\hyperref[app:ablation]{\textit{C.2\; Zero Graph Edges}}
  & \pageref{app:ablation} \\
\quad\hyperref[app:ablation]{\textit{C.3\; No GAT Training (Raw CLIP EOS Embeddings)}}
  & \pageref{app:ablation} \\
\quad\hyperref[app:ablation]{\textit{C.4\; Random Attribute Selection}}
  & \pageref{app:ablation} \\
\quad\hyperref[app:ablation]{\textit{C.5\; Hyperparameter Sensitivity ($\alpha$, $\beta$)}}
  & \pageref{app:ablation} \\[4pt]

% ── Prompt Layout ─────────────────────────────────────
\hyperref[tab:prompt_breakdown]{\textbf{D\; Prompt Token Layout}}
  & \pageref{tab:prompt_breakdown} \\[4pt]
  
% ── Notation ──────────────────────────────────────────
\hyperref[tab:notations]{\textbf{E\; Notation Reference}}
  & \pageref{tab:notations} \\[4pt]
  
\midrule
\multicolumn{2}{@{}l}{\textbf{Figures}} \\[2pt]

\hyperref[fig:tca_pipeline]{TCA Pipeline Overview}
  & \pageref{fig:tca_pipeline} \\
\hyperref[fig:reliability-all]{Reliability Diagrams Across All Datasets (ViT-B/16)}
  & \pageref{fig:reliability-all} \\[4pt]

\midrule
\multicolumn{2}{@{}l}{\textbf{Tables}} \\[2pt]

\hyperref[tab:attr_comparison]{Attribute Comparison: TCA vs.\ \ARGTCADiv{} vs.\ \ARGTCADisc{}}
  & \pageref{tab:attr_comparison} \\
\hyperref[tab:ablation]{Ablation Results}
  & \pageref{tab:ablation} \\
  
\hyperref[tab:prompt_breakdown]{Prompt Token Layout — \ARGTCA{}}
  & \pageref{tab:prompt_breakdown} \\
\hyperref[tab:notations]{Notation Reference}
  & \pageref{tab:notations} \\

\bottomrule
\end{tabular}
\end{table*}
